# Supplementary material for: Language Model Pre-Training with Sparse Latent Typing
Source: arXiv:2210.12582 source file (2022-10-26)
Supplement: Supplementary file 1 [file 7appendix.tex]

% \section{Hyper Parameter Settings}
% \begin{table}[htbp]
% 	\centering
%     \small
% 	\begin{tabular}{cc}
% 		\toprule[1pt] 
% 		Hyper-parameters & Values\\
% 		\midrule[1pt]
% 		Entity embedding dimensions & 768\\
% 		Relation embedding dimensions & 768\\
% 		Event embedding dimensions & 768\\
% 		Event type embedding dimensions & 200\\
% 		Role type embedding dimensions & 200\\
% 		\specialrule{0em}{1pt}{1pt}
% 		\hline
% 		\specialrule{0em}{1pt}{1pt}
%         Event-event passing level $\gamma$ & 0.5  \\
%         Entity-event passing level $\epsilon$ & 0.8  \\
%         \specialrule{0em}{1pt}{1pt}
% 		\hline
%         \specialrule{0em}{1pt}{1pt}
%         Num of layers for FFNNs & 2 \\
%         FFNN hidden dimensions for entity classification & 200 \\
%         FFNN hidden dimensions for relation classification & 200 \\
%         FFNN dropout rate & 0.3 \\
%         GCN dropout rate & 0.4 \\
%         Hidden activation function & \emph{ReLU} \\
%         \specialrule{0em}{1pt}{1pt}
% 		\hline
%         \specialrule{0em}{1pt}{1pt}
%         Learning rate & 1e-4 \\
%         Pretraining batch size & 128 \\
%         Batch size for entity typing & 2,560 \\
%         Batch size for relation typing & 2,560 \\
% 		\midrule[1pt]
% 	\end{tabular}
% 	\normalsize
% 	\caption{Detailed settings for model hyper-parameters. Note that the message passing level $\gamma$ and $\epsilon$ are determined by grid search in the range $[0.1,0.2,0.3,0.4,0.5,0.6,0.7,0.8,0.9,1.0]$.}
% 	\label{tab:parameters}
% \end{table}

% % \section{Entity and Relation Type Categories}
% % \subsection{ACE-2005 Dataset}
% % \paragraph{Entity Types}
% % There are 
